# Supplementary material for: Half-sibling regression meets exoplanet imaging: PSF modeling and subtraction using a flexible, domain knowledge-driven, causal framework
Source: arXiv:2204.03439 source file (2022-04-07)
Supplement: Supplementary file 1 [file half-sibling-regression.tex]

\documentclass[crop, tikz]{standalone}

\usepackage[T1]{fontenc}
\usepackage[utf8]{inputenc}

% Replace ugly default font
\usepackage[varg]{txfonts}

\usepackage{amsmath}
\usepackage{bm}

\usepackage{tikz}
\usetikzlibrary{
    calc,
    decorations.text,
    arrows,
    positioning,
}

\begin{document}
\begin{tikzpicture}[auto, >=stealth']

    \tikzstyle{circ}=[draw=black, very thick, circle, minimum size=1.0cm, inner sep=0, anchor=center, font=\bfseries]
    \tikzstyle{arr}=[->, very thick, draw=black]
    \tikzstyle{annot}=[text=black!50, font=\scriptsize, align=center]

    \draw [fill=white, draw=none] (-8, -3) rectangle (8, 1.5);

    \node [circ, draw=black] at (0, 0) (N) {N};

    \node [circ, left=3cm of N,  draw=black] (Q) {Q};
    \node [circ, below=0.75cm of Q, draw=black] (Y) {Y};
    \node [circ, below=0.75cm of N, draw=none] (M) {};
    \node [circ, right=3cm of N, draw=black!50, text=black!50] (R) {R};
    \node [circ, right=3cm of M, draw=black] (X) {X};
    
    \node [above=2mm of Q, annot] {Flux from\\ exoplanet};
    \node [above=2mm of N, annot] {Systematic noise\\ (e.g., stellar halo, speckles)};
    \node [above=2mm of R, annot, text=black!50] {Stochastic noise\\ (e.g., read-out noise)};
    \node [below=2mm of Y, annot] {Pixel containing noise\\ and exoplanet signal};
    \node [below=2mm of X, annot] {Pixel(s) containing\\ only noise};

    \node [left=1cm of Q, align=right, anchor=east, font=\bfseries] 
        (unobserved) {unobserved:};
    \node [left=1cm of Y, align=right, anchor=east, font=\bfseries] 
        (observed) {observed:};

    \draw [arr] (Q) edge (Y);
    \draw [arr] (N) edge node [midway, above=2mm] {g} (X);
    \draw [arr] (N) edge node [midway, above=2mm] {f} (Y);
    \draw [arr, draw=black!50, fill=black!50] (R) edge (X);
    
    \draw [arr, draw=black!50, loosely dotted, line cap=round, shorten >=0.2cm, shorten <=0.2cm] 
        (X) to [out=200, in=345] (Y);
    \draw[draw=none, fill=white] (-1.95, -2.8) rectangle (2.0, -2.0);
    \draw [decorate, black!50, decoration={text effects along path, text={Idea: learn model {$m$} to predict {$Y$} from {$\bm{X}$}}, text align=center, text effects/.cd, text along path, every character/.style={color=black!50, font=\scriptsize, yshift=-0.55ex}}] (Y) to [out=345, in=200]  (X);

\end{tikzpicture}
\end{document}
